# Supplementary material for: Combining transition path sampling with data-driven collective variables through a reactivity-biased shooting algorithm
Source: arXiv:2404.02597 ancillary file (2024-04-03)
Supplement: Supplementary file 1 [file supporting.pdf]

# Supporting Information

## Combining transition path sampling with data-driven collective variables through a reactivity-biased shooting algorithm

Jintu Zhang,[†,‡] Odin Zhang,[†] Luigi Bonati,[*,‡] and TingJun Hou[*,†,¶]

†*Innovation Institute for Artificial Intelligence in Medicine of Zhejiang University, College of Pharmaceutical Sciences, Zhejiang University, Hangzhou 310058 Zhejiang, China*

‡*Atomistic Simulations, Italian Institute of Technology, Genova 16152, Italy*

¶*State Key Lab of CAD&CG, Zhejiang University, Hangzhou, Zhejiang 310058, China*

E-mail: luigi.bonati@iit.it; tingjunhou@zju.edu.cn

# Appendix: free energy calculations

Free energy profiles for rare events can be effectively reconstructed using CV-based enhanced sampling methods. They work by introducing an external bias potential $V(\mathbf{s})$ which depends on the atomic coordinates $\mathbf{R}$ via the CVs $s = s(\mathbf{R})$. The role of the bias is to enhance the fluctuations of the selected degrees of freedom and accelerate their sampling by lowering the corresponding free energy barriers. In particular, here we used the On-the-fly Probability Enhanced Sampling (OPES) method,[1] which is an improved version of the well-known Metadynamics algorithm.[2] In OPES, instead of constructing the bias $V(\mathbf{s})$ on the fly, the probability distribution at equilibrium $P(\mathbf{s})$ is first reconstructed using a Gaussian kernel density estimator (KDE) and a reweighting procedure. Then, a bias is designed to drive the

system toward a given target distribution $p^{tg}(\mathbf{s})$, such as:

$$V(\mathbf{s}) = -\frac{1}{\beta}\log\frac{p^{tg}(\mathbf{s})}{P(\mathbf{s})}. \tag{1}$$

In the standard `OPES_METAD` method as implemented in PLUMED,[3] the target distribution is chosen to be the well-tempered one: $p^{tg}(\mathbf{s}) \propto P(\mathbf{s})^{\frac{1}{\gamma}}$, in which the equilibrium probability distribution is broadened and the free energy barriers are lowered by a bias factor $\gamma$.[4] Of course, other choices for the target distribution are possible, including the uniform one, those associated with generalized ensembles, and the one associated with the Adaptive Umbrella Sampling scheme.[5]

# Computational Details

## Brownian Particle on 2-Dimensional Potential Energy Surface.

In this work, the $B$ parameter in Eq. 12 from the main text was chosen as 7.5 kJ/mol, while the mass and friction coefficient of the Brownian particle were set to 1 a.m.u. and 20 ps$^{-1}$, correspondingly. These parameters lead to a fast transition process that conventional MD runs could sample. The MD propagations were carried out under a temperature of 300 K using the OpenMM[6] package (version 8.0) with the Langevin integrator[7] provided by OpenMMTools,[8] and the integration time step was set to 2 fs. In all simulations, the trajectories were saved every 10 fs.

We used a neural network with two hidden layers and a 2-32-16-1 architecture for the TPI-DeepTDA CV and the encoder of the multitask CV. The reversed architecture was used as the decoder of the multitask CV. Input features of the network are $X$ and $Y$ positions of the particle. The Adam optimizer was used to optimize both CV, with an initial learning rate of 1E-3 and a $L^2$ regularization term that contains a hyperparameter of 1E-5. In the TPI-DeepTDA CV, the target mean and width of distributions corresponding to the three states

(metastable state A, B and the transition state) were selected as $\mu_A = -10.0$, $\mu_B = 10.0$, $\mu_{TS} = 0.0$ and $\sigma_A = 0.1$, $\sigma_B = 0.1$, $\sigma_{TS} = 4.0$. Similarly, in the auxiliary TDA loss function of the multitask CV, the target means and width of distributions corresponding to the two states (metastable state A, B) were selected as $\mu_A = -10.0$, $\mu_B = 10.0$ and $\sigma_A = 0.2$, $\sigma_B = 0.2$. The weight factor of the auxiliary TDA loss was set as 2.0. The optimization of all MLCVs are performed using the `mlcolvar` python library.[9]

## Alanine Dipeptide.

We used the CHARMM22 force field[10] for simulating alanine dipeptide and the TIP3P water molecules. All chemical bonds involving hydrogen atoms were constrained using the RATTLE[11] algorithm. The electrostatic interactions were described using the Particle Mesh Ewald (PME)[12] method with a real-space cutoff at 1.15 nm. The Lennard-Jones (LJ) interactions were calculated with a distance cutoff of 1.15 nm, The MD propagations were carried out under the NVT ensemble of 300 K using the OpenMM[6] package with the Geodesic BAOAB Langevin integrator[13] provided by OpenMMTools.[8] The integration time step and the friction coefficient were set to 2 fs and 1 ps$^{-1}$, correspondingly. The number of geodesic drift steps was set to 2. In all simulations, the trajectories were saved every 20 fs.

We used a neural network with two hidden layers and a 45-4-2-1 architecture for the TPI-DeepTDA CV and the encoder of the multitask CV. The reversed architecture was used as the decoder of the multitask CV. Input features of the network are the distances between all non-hydrogen atoms of alanine dipeptide. The Adam optimizer was used to optimize both CV, with an initial learning rate of 1E-3 and a $L^2$ regularization term that contains a hyperparameter of 1E-5. In the auxiliary TDA loss function of the multitask CV, the target means and width of distributions corresponding to the two states (metastable state A, B) were selected as $\mu_A = -10.0$, $\mu_B = 10.0$ and $\sigma_A = 1.0$, $\sigma_B = 1.0$. The weight factor of the auxiliary TDA loss was set as 1.0.

In the OPES simulations, we used a barrier parameter of 40 kJ/mol, and the kernel

functions were deployed every 500 steps. We used 0.4 and 0.3 as the initial widths of the kernels in the multitask CV and torsion angles CV-based simulations, correspondingly. All the free energy calculations were performed with the community-developed plugin for molecular dynamics (PLUMED),[3] version 2.9.0.

**Hydrolysis of Acetyl Chloride.**

The simulated system is composed of one acetyl chloride molecule and 53 water molecules and has a size of 1.2×1.2×1.2 nm. The density of the simulation box is about 1 g/cm$^3$. Before *ab initio* MD (AIMD) simulations, the system was minimized and equilibrated for 1 ns using the CHARMM general force filed (CGenFF)[14,15] and the OpenMM[6] package. The *ab initio* calculations were carried out under the density functional theory level using the SIESTA[16,17] package, version 4.1.5. The revPBE functional[18] and the Troullier-Martins FHI98pp norm-conserving[19] pseudopotentials were adopted for the calculations. The pseudopotentials and the accessory double-zeta polarization basis set used in this work were optimized by SIMUNE.[20] In all *ab initio* calculations, a mesh cutoff of 300 Ry was adopted, and the k-point mesh only included the gamma point of the Brillouin zone. Besides, Grimme's D3 correction[21] was added to correct the dispersion interactions.

The initial *ab initio* SMD simulation was performed under the NVT ensemble of 350 K using the SOMD[22] package with a BAOAB Langevin integrator.[23] The integration time step and the friction coefficient were set to 1 fs and 10 ps$^{-1}$, correspondingly. During the 25 ps SMD run, the distance between the chloride atom and the carbon atom that bonds with it was gradually stretched from 0.18 nm to 0.4 nm. We randomly selected 300 structures from the SMD trajectory as the seminal training set and trained an initial NEP using the GPUMD[24] package (version 3.9). Then, using the initial NEP, we performed five successive active learning runs, all performed with SOMD and the `nep` utility of GPUMD. Table S1 (stage 1 to stage 5) summarizes the detailed parameters of these active learning runs.

In these five active learning runs, we used the same SMD setup as in the initial SMD

Table S1: Parameters of different active learning runs.

| Stage | Temperature | Bias Type | MSD_F[a] | # Steps [b] | # Structures [c] | $l_{max}$[d] |
|---|---|---|---|---|---|---|
| 1[e] | 500 K | None | 300 - 500 | 1E5 * 20 * 2 | 50 * 2 | 4 2 |
| 2[f] | 500 K | None | 300 - 500 | 1E5 * 20 * 2 | 50 * 2 | 4 2 |
| 3 | 400 K | SMD | 200 - 500 | 2.5E5 * 12 * 2 | 100 * 2 | 4 2 |
| 4 | 300 K | SMD | 200 - 400 | 2.5E5 * 12 * 3 | 100 * 3 | 4 2 |
| 5 | 300 K | SMD | 200 - 400 | 2.5E5 * 12 * 2 | 100 * 2 | 4 2 1 |
| 6 | 300 K | MetaD | 200 - 400 | 2E6 * 4 * 2 | 100 * 2 | 4 2 1 |

[a] The force MSD range of candidate structures in units of kJ/mol/nm.
[b] Number of MD propagation steps in each active learning run. The three numbers in the expressions stand for the number of steps in one MD run, the number of MD runs in one learning iteration, and number of learning iterations, correspondingly.
[c] Number of candidate structures harvested in each active learning run. The two numbers in the expressions stand for the number of candidate structures in one learning iteration and the number of learning iterations.
[d] The $l_{max}$ parameter (maximum expansion order for the angular terms) used for the trained NEP.[25]
[e] Sampled under the reactant state.
[f] Sampled under the product state.

simulation. Four NEPs were trained from different initial network weights during each learning iteration. In addition to the $l_{max}$ parameter listed in Table S1, the used NEP parameters are as follows. The radial descriptors are composed of 6 radial functions (each being a linear combination of 12 basis functions) that contain a cutoff radius of 0.8 nm. The angular descriptors are composed of 6 radial functions (each being a linear combination of 12 basis functions) that contain a cutoff radius of 0.6 nm. The neural network in the NEP model has a single hidden layer, and 20 neurons were used for this layer. Each NEP was trained for 70000 generations.

After the five active learning runs, we performed a primitive RB-shooting TPS to build the MLCV for the reaction, as mentioned in the main text. We used a neural network with two hidden layers and a 7-8-4-1 architecture for the TPI-DeepTDA CV and the encoder of the multitask CV. The reversed architecture was used for the decoder of the multitask CV. Input features of the network are the distances between all non-hydrogen atoms in the acetyl chloride molecule plus the water coordination number of the carbon atom in the acyl

chloride group. In calculations of the coordination number, the cutoff radius, $NN$, and $MM$ parameters were set to 0.165 nm, 6, and 12 correspondingly. The Adam optimizer was used to optimize both CV, with an initial learning rate of 1E-3 and a $L^2$ regularization term that contains a hyperparameter of 1E-5. In the auxiliary TDA loss function of the multitask CV, the target mean and width of distributions corresponding to the two states (metastable state A, B) were selected as $\mu_A = -10.0$, $\mu_B = 10.0$ and $\sigma_A = 0.25$, $\sigma_B = 0.25$. The weight factor of the auxiliary TDA loss was set as 2.0. Besides, to avoid the Langevin process violating the system's true dynamics, we used the middle-point splitting[26] CSVR thermostat[27] during the TPS simulations. The time step, temperature, and relaxation time of the thermostat were set to 1 fs, 300 K, and 0.1 ps, correspondingly.

With the fitted MLCV and NEP, we carried out an additional active learning run (stage 6 in Table S1) with a WT-MetaD biasing potential. During the MD propagation phase, Gaussian potentials with an initial height of 2.0 kJ/mol and a width of 0.15 CV unit were deployed every 20 steps, and the bias factor was set to 50.

After the above training stages, we obtained a training set of 1400 structures. To avoid possible poor descriptions of the transition state,[28] we selected 200 TS structures from the WT-MetaD trajectories in training stage 6. Here, we again exploited the shooting range optimized from the previous RB-shooting run to identify the TS geometry: if the CV value of a structure is located in the shooting range, it would be considered a TS structure. We trained the final NEP model using the accumulated training set with 1600 structures. In the final training, we changed the number of radial and angular descriptors to 10 and 8 and increased the number of neurons to 36. Other parameters were kept untouched. After 200000 generations of training we tested the accuracy of the model: the root-mean-square errors (RMSEs) for energy and force are 1.2 meV/atom and 0.626 eV/nm in the training dataset.

With the final NEP, we performed the production RB-shooting TPS run, where the setup in the primitive RB-shooting TPS simulation was adopted again. After two biasing function

optimization iterations, we saved the MLCV and performed umbrella sampling free energy calculations. The reaction coordinate was sampled by 39 independent restrained simulations, and each simulation was repeated three times to evaluate the sampling error. The force constant of restraints was selected as 750 kJ/mol/nm, which gives sufficient overlaps between different histograms. All simulations were performed under the NVT ensemble of 300 K with a BAOAB Langevin integrator, the length of each simulation was 500 ps. The integration time step and the friction coefficient were set to 0.5 fs and 10 $ps^{-1}$, correspondingly. After the simulations, the free energies of each window were combined using the weighted histogram analysis method (WHAM). In all above calculations, the biasing potentials were applied using PLUMED (version 2.9.0).

# Supplementary Figures

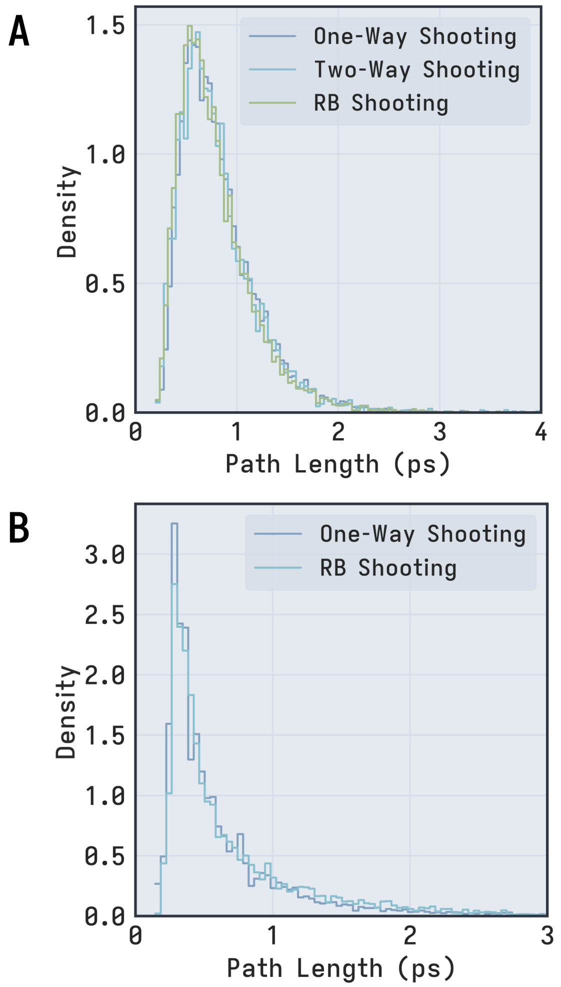


Figure S1: (A) Path lengths distributions of the alanine dipeptide configuration transition process. (B) Path lengths distributions of the hydrolysis reaction of acetyl chloride.

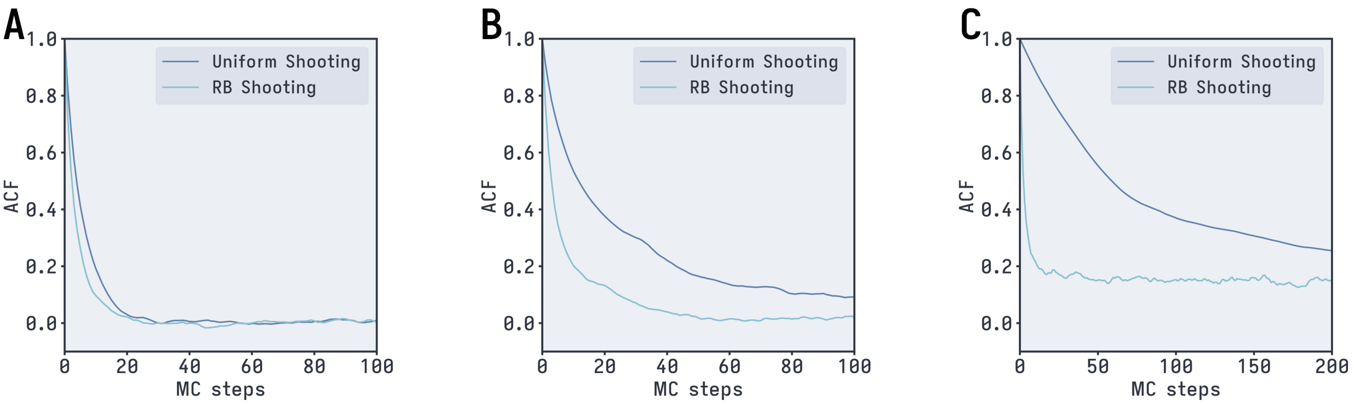


Figure S2: (A) Normalized autocorrelation function (ACF) of the path length v.s. the number of Monte Carlo (MC) steps for the 2D toy system. (B) Normalized autocorrelation function (ACF) of the path length v.s. the number of Monte Carlo (MC) steps for the alanine dipeptide configuration transition process. (C) Normalized autocorrelation function (ACF) of the path length v.s. the number of Monte Carlo (MC) steps for the hydrolysis reaction of acetyl chloride.

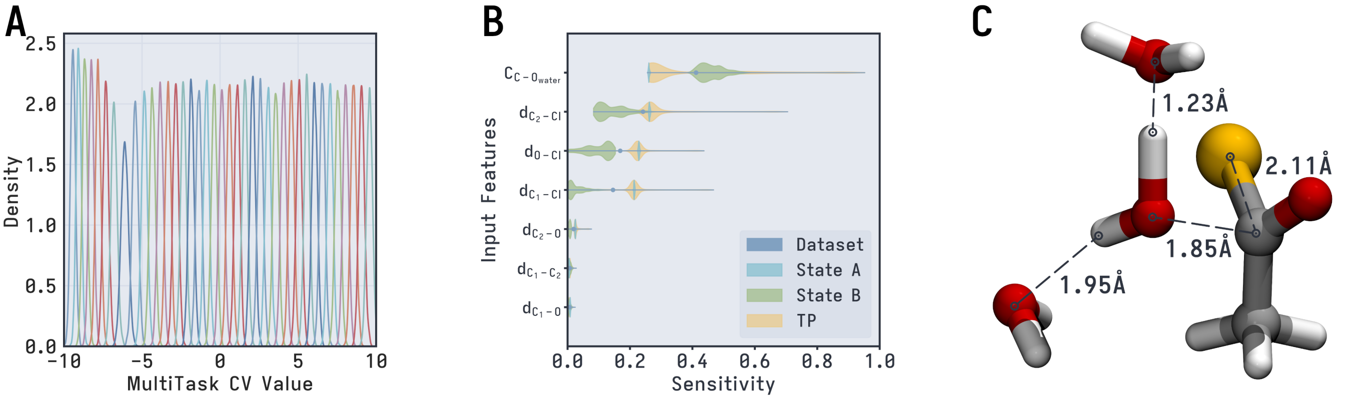


Figure S3: Auxiliary data of the hydrolysis reaction of acetyl chloride. (A) Histograms of the umbrella sampling calculations. (B) Sensitivity analysis of the input descriptors. (C) Averaged transition state structure.

# References


(1) Invernizzi, M.; Parrinello, M. Rethinking Metadynamics: From Bias Potentials to Probability Distributions. *The Journal of Physical Chemistry Letters* **2020**, *11*, 2731–2736, PMID: 32191470.

(2) Laio, A.; Parrinello, M. Escaping free-energy minima. *Proceedings of the National Academy of Sciences* **2002**, *99*, 12562–12566.

(3) The PLUMED consortium et al. Promoting transparency and reproducibility in enhanced molecular simulations. *Nature Methods* **2019**, *16*, 670–673.

(4) Barducci, A.; Bussi, G.; Parrinello, M. Well-Tempered Metadynamics: A Smoothly Converging and Tunable Free-Energy Method. *Phys. Rev. Lett.* **2008**, *100*, 020603.

(5) Invernizzi, M.; Piaggi, P. M.; Parrinello, M. Unified Approach to Enhanced Sampling. *Phys. Rev. X* **2020**, *10*, 041034.

(6) Eastman, P.; Swails, J.; Chodera, J. D.; McGibbon, R. T.; Zhao, Y.; Beauchamp, K. A.; Wang, L.-P.; Simmonett, A. C.; Harrigan, M. P.; Stern, C. D.; others OpenMM 7: Rapid development of high performance algorithms for molecular dynamics. *PLoS computational biology* **2017**, *13*, e1005659.

(7) Bussi, G.; Parrinello, M. Accurate sampling using Langevin dynamics. *Phys. Rev. E* **2007**, *75*, 056707.

(8) Chodera, J. et al. choderalab/openmmtools: 0.23.1. 2023; `https://doi.org/10.5281/zenodo.8102771`.

(9) Bonati, L.; Trizio, E.; Rizzi, A.; Parrinello, M. A unified framework for machine learning collective variables for enhanced sampling simulations: mlcolvar. *The Journal of Chemical Physics* **2023**, *159*, 014801.

(10) Mackerell Jr., A. D.; Feig, M.; Brooks III, C. L. Extending the treatment of backbone energetics in protein force fields: Limitations of gas-phase quantum mechanics in reproducing protein conformational distributions in molecular dynamics simulations. *Journal of Computational Chemistry* **2004**, *25*, 1400–1415.

(11) Andersen, H. C. Rattle: A "velocity" version of the shake algorithm for molecular dynamics calculations. *Journal of Computational Physics* **1983**, *52*, 24–34.

(12) Essmann, U.; Perera, L.; Berkowitz, M. L.; Darden, T.; Lee, H.; Pedersen, L. G. A smooth particle mesh Ewald method. *The Journal of Chemical Physics* **1995**, *103*, 8577–8593.

(13) Leimkuhler, B.; Matthews, C. Efficient molecular dynamics using geodesic integration and solvent–solute splitting. *Proceedings of the Royal Society A: Mathematical, Physical and Engineering Sciences* **2016**, *472*, 20160138.

(14) Vanommeslaeghe, K.; Hatcher, E.; Acharya, C.; Kundu, S.; Zhong, S.; Shim, J.; Darian, E.; Guvench, O.; Lopes, P.; Vorobyov, I.; Mackerell Jr., A. D. CHARMM general force field: A force field for drug-like molecules compatible with the CHARMM all-atom additive biological force fields. *Journal of Computational Chemistry* **2010**, *31*, 671–690.

(15) Yu, W.; He, X.; Vanommeslaeghe, K.; MacKerell Jr., A. D. Extension of the CHARMM general force field to sulfonyl-containing compounds and its utility in biomolecular simulations. *Journal of Computational Chemistry* **2012**, *33*, 2451–2468.

(16) Soler, J. M.; Artacho, E.; Gale, J. D.; García, A.; Junquera, J.; Ordejón, P.; Sánchez-Portal, D. The SIESTA method for ab initio order-N materials simulation. *Journal of Physics: Condensed Matter* **2002**, *14*, 2745.

(17) García, A. et al. Siesta: Recent developments and applications. *The Journal of Chemical Physics* **2020**, *152*, 204108.

(18) Zhang, Y.; Yang, W. Comment on "Generalized Gradient Approximation Made Simple". *Phys. Rev. Lett.* **1998**, *80*, 890–890.

(19) Fuchs, M.; Scheffler, M. Ab initio pseudopotentials for electronic structure calculations of poly-atomic systems using density-functional theory. *Computer Physics Communications* **1999**, *119*, 67–98.

(20) Oroya, J.; Callejo, M.; Garcia-Mota, M.; Marchesin, F. Pseudopotential and Numerical Atomic Orbitals Basis Dataset. *An online database of numerical atomic orbitals compatible with the Siesta code* **2020**, *257*.

(21) Grimme, S.; Antony, J.; Ehrlich, S.; Krieg, H. A consistent and accurate ab initio parametrization of density functional dispersion correction (DFT-D) for the 94 elements H-Pu. *The Journal of Chemical Physics* **2010**, *132*, 154104.

(22) SOMD. `https://github.com/initqp/somd`, 2023.

(23) Leimkuhler, B.; Matthews, C. Rational Construction of Stochastic Numerical Methods for Molecular Sampling. *Applied Mathematics Research eXpress* **2012**, *2013*, 34–56.

(24) Fan, Z. et al. GPUMD: A package for constructing accurate machine-learned potentials and performing highly efficient atomistic simulations. *The Journal of Chemical Physics* **2022**, *157*, 114801.

(25) Fan, Z. Improving the accuracy of the neuroevolution machine learning potential for multi-component systems. *Journal of Physics: Condensed Matter* **2022**, *34*, 125902.

(26) Zhang, Z.; Liu, X.; Chen, Z.; Zheng, H.; Yan, K.; Liu, J. A unified thermostat scheme for efficient configurational sampling for classical/quantum canonical ensembles via molecular dynamics. *The Journal of Chemical Physics* **2017**, *147*, 034109.

(27) Bussi, G.; Donadio, D.; Parrinello, M. Canonical sampling through velocity rescaling. *The Journal of Chemical Physics* **2007**, *126*, 014101.

(28) Yang, M.; Bonati, L.; Polino, D.; Parrinello, M. Using metadynamics to build neural network potentials for reactive events: the case of urea decomposition in water. *Catalysis Today* **2022**, *387*, 143–149, 100 years of CASALE SA: a scientific perspective on catalytic processes.
